# Supplementary material for: Beyond Counting Datasets: A Survey of Multilingual Dataset Construction and Necessary Resources
Source: arXiv:2211.15649 source file (2022-11-28)
Supplement: Supplementary file 2 [file appendix_scheme_shorten.tex]

\vspace{-0.5em}
\begin{table}[ht!]
\small
    \centering
        \begin{tabular}{p{1.5cm}|p{6.5cm}}\toprule
        Aspect & Categories \\ \midrule
        Language & ISO 639-1 Language Code \\ \midrule
        Task type & classification (sentiment analyis). classification (sentence pair),classification (other), QA (w/ retrieval), QA (machine reading), structured prediction, sequence tagging, generation (summarization), generation (other), other\\ \midrule
        Dataset size & $< 100$, $100\sim 1000$, $1000\sim10k$, $> 10k$ \\ \midrule
        Train data & yes / no / partial / not mentioned \\ \midrule
        Creator & industry, individual researchers, university, and combination of the above \\ \midrule
        Pub. Venue & *CL, *ACL Workshop, Findings, NeurIPS Datasets and Benchmarks Track, arXiv, N/A\\ \midrule
        Pub.  Year & Year of publication \\ \midrule
        Motivation & cross-lingual transfer, single task (multilingual) w/ ML training, single task (single lang), multi-task (single lang)\\ \midrule
        {$x$ source}& annotated (authors, linguists), commercial sources, crowdsourced, curated linguistic resources, curated source, media, template-based, web, wikipedia, and combination of the above\\ \midrule
        $x$ language& English, in its own language, both, other language, not mentioned\\ \midrule
        $y$ collection & annotated (authors, linguists), automatically induced, crowdsourced, curated linguistic resources, not mentioned, and combination of the above\\ \midrule
        $y$ Language& English, its own language, not mentioned\\\midrule
        Reuse & yes (English), yes (other language), yes (English \& other language), no reuse\\\midrule
        Translation& automatic translation, human (author), human (non-author), no translation, unclear \\ 
        \bottomrule
    \end{tabular}
    \vspace{-0.5em}
    \caption{Full Annotation Scheme.}
    \label{tab:annot_scheme}
\end{table}
